# Supplementary material for: Semantically Aligned Gradient-Driven Context-Preserving Image Editing
Source: arXiv:2609.12691 source file (2026-09-11)
Supplement: Supplementary file 1 [file supplementary_root.tex]

\documentclass[runningheads]{llncs}

% Review version (uncomment and set ID as needed):
% \usepackage[review,year=2026,ID=14030]{eccv}
\usepackage{eccv}

\usepackage{amsmath,amssymb}
\usepackage{graphicx}
\usepackage{booktabs}
\usepackage[table]{xcolor}
\usepackage{orcidlink}

\definecolor{lightred}{RGB}{255,220,220}
\definecolor{darkgreen}{RGB}{0,100,0}

% eccv loads hyperref; configure it
\hypersetup{colorlinks=true,linkcolor=blue,citecolor=blue,urlcolor=blue}

\begin{document}
\input{supplementary}
\end{document}
